# Supplementary material for: RuleR: Improving LLM Controllability by Rule-based Data Recycling
Source: arXiv:2406.15938 source file (2025-02-15)
Supplement: Supplementary file 1 [file appendix_related_work.tex]

\section{Realted Work}
\subsection{Controllability of LLM } In recent research, the controllability of LLM is becoming increasingly significant in evaluating the performance of large language models~\cite{sun2024conifer, xia2024fofo, zhou2023instructionfollowing,chen2024benchmarking,qin2024infobench}. 
According to the systematic investigation from \citet{Liu_2024}, it is essential for LLMs to constrain their outputs to follow specific user-defined formats or standards. 
IFEval~\cite{zhou2023instructionfollowing} proposed the concept of "verifiable instruction," which details the constraints on response behaviors within the instruction. This approach standardizes and simplifies the evaluation process of the instruction-following capabilities of LLMs.  FOFO~\cite{xia2024fofo} discovered that the ability to follow the format constraints is independent of content generation and varies across different domains. Evaluation benchmarks were constructed using the "Domain-subdomain-format" framework to specifically assess the controllability.
InFoBench~\cite{qin2024infobench} developed an evaluation framework that decomposes complex instructions into constraint-based yes/no questions. This approach provides clearer insights into a model's ability to follow instructions, particularly in complex scenarios. The evaluation instructions chosen encompass not only content constraints but also include style rules, format specifications, and number limitations.
CoDI-Eval~\cite{chen2024benchmarking} proposed automated and easy-to-use benchmarks to evaluate the performance of LLMs in following constraint-based instructions. The evaluation tasks in CoDI-Eval encompass sentiment analysis, topic identification, keyword extraction, length constraints, and toxicity avoidance. These tasks are designed to create a diverse and controllable benchmark for comprehensive performance assessment.
